# Supplementary material for: ReconfigISP: Reconfigurable Camera Image Processing Pipeline
Source: arXiv:2109.04760 source file (2021-09-10)
Supplement: Supplementary file 1 [file appendix.tex]

% !TEX root = ../submission.tex
% Appendix
\appendix
\section{High-Level To-Do List}
\begin{enumerate}
	\item Basic modules
	\begin{enumerate}
		\item BM3D
		\item Path-Restore
		\item Local tone mapping
		\item Bayer denoising methods
	\end{enumerate}
	\item General ISP with limited training data
	\begin{enumerate}
		\item SIDD dataset (denoising)
		\item SID dataset (extremely dark scenes)
		\item S7 ISP dataset (normal scenes)
	\end{enumerate}
	\item Task-specific ISP with limited training data
	\begin{enumerate}
		\item Data collection and annotation
	\end{enumerate}
	\item Runtime-constrained ISP. May use the same datasets as (2)
\end{enumerate}

\section{Detailed To-Do List}
\begin{enumerate}
	\item Basic modules
	\begin{enumerate}
		\item BM3D
		\begin{enumerate}
			\item Specify parameters [\zx]
			\item Generate training data [\zx]
			\item Proxy training [\ke, \zx]
		\end{enumerate}
		\item Path-Restore
		\begin{enumerate}
			\item Train a model in Bayer domain [\ke]
			\item TensorFlow -> PyTorch with certain paths [\ke]
		\end{enumerate}
		\item Local tone mapping
		\begin{enumerate}
			\item Basic algorithm [\yue]
			\item Data generation [\ke, \zx]
			\item Proxy training [\ke, \zx]
		\end{enumerate}
		\item Bayer denoising methods (consider channel correlations?)
		\begin{enumerate}
			\item Basic algorithm [\yue]
			\item Data generation [\ke, \zx]
			\item Proxy training [\ke, \zx]
		\end{enumerate}
		\item Sharpness and contrast modules [\yue, \ke]
	\end{enumerate}
	\item General ISP with limited training data
	\begin{enumerate}
		\item SIDD dataset (denoising)
		\begin{enumerate}
			\item Our method [\ke]
		\end{enumerate}
		\item SID dataset (extremely dark scenes)
		\begin{enumerate}
			\item Our method [\ke]
			\item See in the Dark with limited data [\ke]
		\end{enumerate}
		\item S7 ISP dataset (normal scenes)
		\begin{enumerate}
			\item Our method [\ke]
			\item See in the Dark with limited data [\ke]
		\end{enumerate}
	\end{enumerate}
	\item Task-specific ISP with limited training data
	\begin{enumerate}
		\item PASCALRAW dataset (not proper)
		%\begin{enumerate}
		%	\item Study the dataset [\ke]
		%	\item Train object detector [\yue, \ke]
		%	\item Our method [\ke]
		%\end{enumerate}
		\item Synthesize data sRGB -> RAW
		\item Data collection and annotation
	\end{enumerate}
	\item Runtime-constrained ISP. May use the same datasets as (2)
	\begin{enumerate}
		\item Evaluate algorithm complexity [\yue]
		\item Our method (may try different loss functions) [\ke]
	\end{enumerate}
	\item Other action items
	\begin{enumerate}
		\item Accelerate I/O speed when trained on clusters [\ke]
		\item Test based on the original ISP modules (not proxy) [\ke]
		\item Run Software ISP on different datasets [\zx]
		\item Survey existing ISP pipelines in industry [\yue]
	\end{enumerate}
\end{enumerate}
